# Supplementary material for: PAC-CF: Calibrating Irreversible Frontier Pruning in LLM-Guided Search
Source: arXiv:2604.14345 source file (2026-10-06)
Supplement: Supplementary file 1 [file supplementary.tex]

\documentclass[11pt, letterpaper]{article}

% --- 基础宏包 ---
\usepackage[utf8]{inputenc}
\usepackage[margin=1in]{geometry}
\usepackage{amsmath,amssymb,amsthm}
\usepackage{enumitem}

% --- 宏定义 (必须和主文保持一致) ---
\newtheorem{theorem}{Theorem}
\newtheorem{lemma}{Lemma}

\newcommand{\E}{\mathbb{E}}
\newcommand{\Prob}{\mathbb{P}}
\newcommand{\F}{\mathcal{F}}

\title{\Large \bf Supplementary Material for:\\ "Tight Sample Complexity Bounds for Best-Arm Identification under Bounded Systematic Bias"}
\author{Tianhao Qian}
\date{}

\begin{document}
\maketitle

\section{Detailed Theoretical Proofs}
\label{sec:appendix_proofs}

In this section, we provide detailed proofs for the theoretical results presented in Section \ref{sec:theory}. We employ $b_m(n)$ to denote the empirical mean of arm $m$ after $n$ samples. Crucially, because our theoretical framework formulates the node expansion step as a localized Best-Arm Identification problem over the dynamic frontier $\mathcal{A}_t$, the bias term $L$ utilized throughout the following lemmas strictly represents the global supremum of the systematic bias within $\mathcal{A}_t$. Since the node elimination mechanism operates exclusively within this active subset, bounding individual node biases by this global supremum preserves the strict validity of all algebraic inequalities without invoking the unrealistic assumption of global error uniformity.

\begin{lemma}[Global Time-Uniform Concentration]
\label{lem:concentration_full}
Let $b_m(n) = \frac{1}{n}\sum_{t=1}^n Y_{m,t}$ be the empirical mean of node $m$ after $n$ samples. For a failure probability $\delta \in (0,1)$ and total nodes $M$, let
\[
u_{\text{stat}}(n, \delta/M) = \sqrt{\frac{2\sigma^2 \ln\left(\frac{\pi^2 n^2 M}{3\delta}\right)}{n}}
\]
Then with probability at least $1-\delta$, for all nodes $m \in \{1, \dots, M\}$ and all times $n \ge 1$:
\[
|b_m(n) - \mu_m| \le u_{\text{stat}}(n, \delta/M) + L
\]
\end{lemma}

\begin{proof}
We start with the triangle inequality decomposition for a single arm $m$ and time $n$:
\[
|b_m(n) - \mu_m| \le \underbrace{|b_m(n) - \E[b_m(n)]|}_{\text{Stochastic Error}} + \underbrace{|\E[b_m(n)] - \mu_m|}_{\text{Systematic Bias}}
\]

It therefore suffices to bound the bias and the stochastic term. By Assumption 1, for any single observation, the conditional bias is bounded by $|\E[Y_{m,t}|\F_{t-1}] - \mu_m| \le L$. Due to the linearity of expectation, the bias of the empirical mean is bounded by the average of the individual biases:

\[
\begin{aligned}
|\E[b_m(n)] - \mu_m| &= \left| \frac{1}{n}\sum_{t=1}^n (\E[Y_{m,t}|\F_{t-1}] - \mu_m) \right| \\
&\le \frac{1}{n}\sum_{t=1}^n L = L.
\end{aligned}
\]

To bound the stochastic term, we first let $\xi_{m,t} = Y_{m,t} - \E[Y_{m,t}|\F_{t-1}]$. Under Assumption 1, $\xi_{m,t}$ constitutes a $\sigma^2$-sub-Gaussian martingale difference sequence. To establish a bound valid for all $n \ge 1$ simultaneously, we employ the \textbf{Method of Mixtures}\cite{howard2021time}.
Consider the exponential supermartingale $M_n(\lambda) = \exp(\sum_{t=1}^n \lambda \xi_{m,t} - \frac{\lambda^2 \sigma^2 n}{2})$. According to \textbf{Ville's Maximal Inequality} , we have for any $\delta' \in (0,1)$:
\[
\Prob(\exists n \ge 1: |S_n| \ge u_{\text{boundary}}(n, \delta')) \le \delta'
\], where $S_n = \sum_{t=1}^n \xi_{m,t}$. 

With the sub-Gaussian boundary $u_{\text{boundary}}(n, \delta') = \sqrt{2\sigma^2 n \ln(\frac{\pi^2 n^2}{3\delta'})}$, normalizing by $n$ yields the desired time-uniform concentration:
\[
\Prob\left(\exists n \ge 1: |b_m(n) - \E[b_m(n)]| \ge u_{\text{stat}}(n, \delta') \right) \le \delta'
\]

Based on these two bounds, we can apply a union bound over M Arms by setting the per-arm failure probability to $\delta' = \delta/M$ so that the bound holds for all $M$ nodes simultaneously:
\[
\begin{aligned}
\Prob\Big(\exists m \in \{1,\dots,M\}: |b_m(n) &- \mu_m| > u_{\text{stat}}(n, \delta/M) + L \Big) \\
&\le \sum_{m=1}^M \frac{\delta}{M} = \delta.
\end{aligned}
\]
Thus, with probability $1-\delta$, the condition holds for all $m$ and all $n$.
\end{proof}

\begin{lemma}[Safety Condition for Proportion-based Pruning]
\label{lem:safety}
Assume the high-probability event $\mathcal{E}$ holds. Let $M_{bad}$ be the set of suboptimal nodes that are distinguishable from the optimal node $m^*$ under the current sample size, satisfying the gap condition:
\[
\forall j \in M_{bad}: \quad \Delta_j > 2L + u_{\text{stat}}(n_{m^*}, \delta/M) + u_{\text{stat}}(n_j, \delta/M).
\]
Let $K = \lfloor a |\mathcal{A}_t| \rfloor$ be the number of nodes to be pruned. If the pruning proportion $a$ is chosen such that:
\[
K \le |M_{bad}|,
\]
then the optimal node $m^*$ is strictly separated from the elimination set and is guaranteed to survive.
\end{lemma}

\begin{proof}
We first condition on event $\mathcal{E}$. By applying the bounds from Lemma \ref{lem:concentration_full}, we lower-bound the empirical difference between $m^*$ and any $j \in M_{bad}$:

\begin{align*}
b_{m^*}(t) - b_j(t) &\ge (\mu^* - u_{\text{stat}}(n_{m^*}) - L) - (\mu_j + u_{\text{stat}}(n_j) + L) \\
&= \Delta_j - 2L - u_{\text{stat}}(n_{m^*}) - u_{\text{stat}}(n_j).
\end{align*}

Under the gap condition for $M_{bad}$, the right-hand side is strictly positive, implying $b_{m^*}(t) > b_j(t)$ holds for all $j \in M_{bad}$.

Since $m^*$ has a strictly higher empirical mean than any node in $M_{bad}$, it is guaranteed a rank strictly above all $|M_{bad}|$ candidates in the sorted list. 

Consequently, combining this ranking with the cardinality constraint $K \le |M_{bad}|$, the set of eliminated nodes (the bottom $K$ positions) corresponds exclusively to indices associated with $M_{bad}$ (or nodes strictly inferior to them). Thus, $m^*$ falls strictly outside the elimination set and is preserved in the next iteration.
\end{proof}

This safety condition inherently provides the formal theoretical justification for dynamic pruning schedules in practical implementations. Intuitively, early in the search when clearly suboptimal nodes abound (i.e., $|M_{bad}|$ is large), a higher pruning rate $a$ is permissible to aggressively accelerate convergence. However, as the candidate set becomes more competitive and the active frontier shrinks, the pruning rate must be dynamically decayed to continually satisfy the constraint $K \le |M_{bad}|$, thereby ensuring the optimal trajectory is never erroneously discarded.

\begin{theorem}[Step-wise PAC Guarantee]
\label{thm:complexity_full}
Consider any expansion step with a frontier set of size $M$. With probability $1-\delta$, Algorithm \ref{alg:pac_mcts} correctly identifies an $\varepsilon$-optimal node $m^*$ to expand. The sample complexity required to distinguish a suboptimal node $m$ from $m^*$ is bounded by:
\[
N_m = O\left( \frac{\sigma^2 \left( \ln(M/\delta) + \ln(\Delta_{eff}^{-2}) \right)}{(\Delta_m - \varepsilon - 4L)^2} \right)
\]
provided the effective gap satisfies $\Delta_{eff} = \Delta_m - 4L > \varepsilon$.
\end{theorem}

\begin{proof}
The algorithm eliminates a suboptimal node $m$ via Confidence-based Pruning (Algorithm \ref{alg:pac_mcts}) when:
\[
b_m(t) + u_{\text{dist}}(n_m) < b_{m^*}(t) - u_{\text{dist}}(n_{m^*}) - \varepsilon
\]
By the definition of the robust confidence radius $u_{\text{dist}}(n) = u_{\text{stat}}(n, \delta/M) + L$, we analyze the worst-case scenario where the empirical means deviate maximally towards each other to find the required sample size. Substituting the bounds from Lemma \ref{lem:concentration_full}:
\begin{itemize}
    \item $b_m(t) \le \mu_m + u_{\text{stat}}(n_m) + L$
    \item $b_{m^*}(t) \ge \mu^* - u_{\text{stat}}(n_{m^*}) - L$
\end{itemize}
The pruning condition is satisfied if the following inequality holds:
\[
\begin{aligned}
(\mu_m &+ u_{\text{stat}}(n_m) + L) + (u_{\text{stat}}(n_m) + L) \\
&< (\mu^* - u_{\text{stat}}(n_{m^*}) - L) - (u_{\text{stat}}(n_{m^*}) + L) - \varepsilon
\end{aligned}
\]
Rearranging the terms and substituting the true suboptimality gap $\Delta_m = \mu^* - \mu_m$, we obtain:
\[
2u_{\text{stat}}(n_m) + 2u_{\text{stat}}(n_{m^*}) < \Delta_m - 4L - \varepsilon
\]
Because tree search algorithms inherently sample nodes highly asymmetrically, we cannot assume uniform visits $n_m \approx n_{m^*}$. Let $n_{\min} = \min(n_m, n_{m^*})$ denote the worst-case minimum sample count between the evaluated nodes. Since the statistical confidence radius $u_{\text{stat}}(n)$ is strictly monotonically decreasing with $n$, it holds that $u_{\text{stat}}(n_m) \le u_{\text{stat}}(n_{\min})$ and $u_{\text{stat}}(n_{m^*}) \le u_{\text{stat}}(n_{\min})$. 

Thus, a sufficient and strictly bounded condition to guarantee safe pruning is:
\[
4u_{\text{stat}}(n_{\min}) < \Delta_m - 4L - \varepsilon
\]
This inequality formally demonstrates that the discriminative power is bottlenecked by the least-sampled node in the active frontier, and the effective gap is explicitly constrained by $\Delta_m - 4L$. If $\Delta_m \le 4L + \varepsilon$, the safety condition can never be guaranteed regardless of the sample size.

To derive the exact sample complexity without loose asymptotic approximations, we must substitute the precise form of the confidence radius $u_{\text{stat}}(n_{\min}) = \sqrt{\frac{2\sigma^2 \ln(C_1 n_{\min}^2)}{n_{\min}}}$ (where $C_1 = \pi^2 M / 3\delta$) into the strict safety condition. This yields a non-linear inequality:$$\frac{n_{\min}}{\ln(C_1 n_{\min}^2)} > C_2$$where the constant is defined as $C_2 = \frac{32 \sigma^2}{(\Delta_m - 4L - \varepsilon)^2}$. To isolate $n_{\min}$ explicitly, we apply the standard transformation $x e^x = y$, which allows us to solve the boundary via the negative branch of the Lambert W function, $W_{-1}$. Applying the established asymptotic expansion $-W_{-1}(-x) \approx \ln(1/x) + \ln(\ln(1/x))$ for $x \to 0^+$, the leading terms directly extract the additive dependencies of $\ln(C_1)$ and $\ln(C_2)$. Substituting $C_1 \propto M/\delta$ and $C_2 \propto (\Delta_m - 4L)^{-2}$, this derivation rigorously generates the exact additive sample complexity:
\[
N_m = O\left( \frac{\sigma^2 \left( \ln(M/\delta) + \ln(\Delta_{eff}^{-2}) \right)}{(\Delta_m - 4L - \varepsilon)^2} \right)
\]
Unlike looser multiplicative envelopes, this precise additive inversion preserves the exact structural order of the sample complexity required to safely prune arm $m$ \cite{kaufmann2016complexity}.
\end{proof}

\begin{theorem}[Lower Bound]
\label{thm:lower_bound_full}
Any algorithm identifying an $\varepsilon$-optimal arm with probability $1-\delta$ under the bounded-bias model satisfies:
\[
\E[N] \ge \Omega\left(\sum_{m \neq m^*} \frac{\sigma^2 \ln(1/\delta)}{(\Delta_m + \varepsilon - 2L)^2}\right)
\]
\end{theorem}

\begin{proof}
We establish this lower bound via a change-of-measure argument. Consider a bandit problem with $M$ arms, and let $\mathbb{P}$ and $\mathbb{Q}$ denote two distinct probability measures corresponding to two hypothetical reward environments.

Under measure $\mathbb{P}$, let arm 1 be optimal with expected true reward $\mu_1$, and arm 2 (representing an arbitrary suboptimal node $m$) have $\mu_2 = \mu_1 - \Delta_m$. The adversary assigns a positive systematic bias $+L$ to arm 2, yielding an observation mean $\E_{\mathbb{P}}[Y_2] = \mu_2 + L$.

Under the alternative measure $\mathbb{Q}$, we construct an environment where arm 2 is the unique $\varepsilon$-optimal arm. We set its true mean to $\mu'_2 = \mu_1 + \varepsilon + \gamma$ (for an arbitrarily small $\gamma > 0$). Here, the adversary assigns a negative systematic bias $-L$ to arm 2, yielding an observation mean $\E_{\mathbb{Q}}[Y_2] = \mu'_2 - L$. The distributions for all other arms remain identical across both measures.

For any algorithm to satisfy the PAC guarantee, it must identify the correct arm with probability at least $1-\delta$ under both measures. By the Bretagnolle-Huber inequality, the Kullback-Leibler (KL) divergence between the observation trajectories must satisfy:
\[
D_{\text{KL}}(\mathbb{P}^{\otimes N} \parallel \mathbb{Q}^{\otimes N}) \ge \ln\left(\frac{1}{4\delta}\right)
\]

Assuming Gaussian noise $\mathcal{N}(0, \sigma^2)$, the KL divergence for arm 2 after $\E[N]$ expected pulls is given by:
\[
D_{\text{KL}}(\mathbb{P}^{\otimes N} \parallel \mathbb{Q}^{\otimes N}) = \E[N] \frac{(\E_{\mathbb{Q}}[Y_2] - \E_{\mathbb{P}}[Y_2])^2}{2\sigma^2}
\]

The analytical distance between the observation means is:
\begin{align*}
\E_{\mathbb{Q}}[Y_2] - \E_{\mathbb{P}}[Y_2] &= (\mu'_2 - L) - (\mu_2 + L) \\
&= (\mu_1 + \varepsilon + \gamma - L) - (\mu_1 - \Delta_m + L) \\
&= \Delta_m + \varepsilon + \gamma - 2L
\end{align*}

Substituting this distance into the KL divergence bound yields:
\[
\E[N] \frac{(\Delta_m + \varepsilon + \gamma - 2L)^2}{2\sigma^2} \ge \ln\left(\frac{1}{4\delta}\right)
\]

Taking the limit as $\gamma \to 0^+$, we obtain the necessary sample complexity for distinguishing arm $m$:
\[
\E[N] \ge \frac{2\sigma^2 \ln(1/4\delta)}{(\Delta_m + \varepsilon - 2L)^2}
\]

Summing this requisite complexity over all suboptimal arms $m \neq m^*$ yields the overall lower bound, mathematically confirming that systematic bias enforces a rigid sample penalty of at least $2L$ on the effective gap.
\end{proof}

\end{document}
